# Supplementary material for: Exploring the Limits of Natural Language Inference Based Setup for Few-Shot Intent Detection
Source: arXiv:2112.07434 source file (2023-12-26)
Supplement: Supplementary file 1 [file appendix.tex]

\section{Dataset}
\label{data_appendix}
% \small
% \renewcommand{\arraystretch}{1.15}

\begin{table*}[ht]
\small
\centering

\begin{tabular}{l|ccccc}
\multicolumn{1}{c|}{\textbf{}}                                                       & \textbf{SNIPS}                                                                                         & \textbf{ATIS}                                                                            & \textbf{NLUED}                                                                                             & \textbf{BANKING77}                                                                                                        & \textbf{CLINC150}                                                                                    \\ \hline
Total Class                                                                          & 7                                                                                                      & 16                                                                                       & 64                                                                                                        & 77                                                                                                                        & 150                                                                                                  \\
Base Class                                                                           & 4                                                                                                      & 12                                                                                       & 46                                                                                                        & 50                                                                                                                        & 100                                                                                                  \\
Novel Class                                                                          & 3                                                                                                      & 4                                                                                        & 16                                                                                                        & 27                                                                                                                        & 50                                                                                                   \\
Vocab Size                                                                           & 8371                                                                                                   & 906                                                                                      & 4232                                                                                                      & 4458                                                                                                                      & 6221                                                                                                 \\
Training Samples                                                                     & 6293                                                                                                   & 4030                                                                                     & 6393                                                                                                      & 5643                                                                                                                      & 10000                                                                                                \\
Test Samples                                                                         & 2688                                                                                                   & 1359                                                                                     & 1871                                                                                                      & 4394                                                                                                                      & 7495                                                                                                 \\
Avg. Utterance Length                                                                     & 9.44                                                                                                   & 11.52                                                                                    & 7.32                                                                                                      & 11.83                                                                                                                     & 8.13                                                                                                 \\
\begin{tabular}[c]{@{}l@{}}Exact match: \\ utterance w/ class-label\end{tabular}     & 0.40\%                                                                                                 & 73.50\%                                                                                  & 0.32\%                                                                                                    & 1.78\%                                                                                                                    & 21.85\%                                                                                              \\
\begin{tabular}[c]{@{}l@{}}Unordered match: \\ utterance w/ class-label\end{tabular} & 9.44\%                                                                                                 & 73.92\%                                                                                  & 3.41\%                                                                                                    & 12.25\%                                                                                                                   & 33.31\%                                                                                              \\ \hline
Example Intents                                                                      & \multicolumn{1}{l}{}                                                                                   & \multicolumn{1}{l}{}                                                                     & \multicolumn{1}{l}{}                                                                                      & \multicolumn{1}{l}{}                                                                                                      & \multicolumn{1}{l}{}                                                                                 \\
\multicolumn{1}{r|}{Base:}                                                           & \multicolumn{1}{l}{\textit{\begin{tabular}[c]{@{}l@{}}book\_restaurant, \\ get\_weather\end{tabular}}} & \multicolumn{1}{l}{\textit{\begin{tabular}[c]{@{}l@{}}capacity, \\ flight\end{tabular}}} & \multicolumn{1}{l}{\textit{\begin{tabular}[c]{@{}l@{}}calendar\_query, \\ qa\_factoid\end{tabular}}}      & \multicolumn{1}{l}{\textit{\begin{tabular}[c]{@{}l@{}}automatic\_top\_up, \\ card\_acceptance\end{tabular}}}              & \multicolumn{1}{l}{\textit{\begin{tabular}[c]{@{}l@{}}pto\_request, \\ food\_last\end{tabular}}} \\
                                                                                     & \multicolumn{5}{l}{}                                     \\
\multicolumn{1}{r|}{Novel:}                                                          & \multicolumn{1}{l}{\textit{\begin{tabular}[c]{@{}l@{}}play\_music, \\ rate\_book\end{tabular}}}        & \multicolumn{1}{l}{\textit{\begin{tabular}[c]{@{}l@{}}meal, \\ quantity\end{tabular}}}   & \multicolumn{1}{l}{\textit{\begin{tabular}[c]{@{}l@{}}general\_negate, \\ alarm\_remove\end{tabular}}} & \multicolumn{1}{l}{\textit{\begin{tabular}[c]{@{}l@{}}card\_about\_to\_expire, \\ reverted\_card\_payment\end{tabular}}} & \multicolumn{1}{l}{\textit{\begin{tabular}[c]{@{}l@{}}rollover\_401k, \\ spelling\end{tabular}}}    \\
\hline
\end{tabular}
\caption{Statistics for different intent datasets. \textit{Training samples} exclude the count of few-shot examples.}
\label{data_stats}
\end{table*}

Table \ref{data_stats} represents the statistical information of all intent datasets along with few examples of base and novel intents for each case. Additionally, we also report the match between tokens of  class-label name and tokens of corresponding utterance for all datasets. \textit{Exact match} refers to the percentage of utterances that contain the class-label name as is, while \textit{unordered match} represents the fraction of utterances where all tokens in class-label name are present in the utterance in any order.

\section{Fine-grained Analysis of Results}
\label{fine_grained}
% It can be noted from Table \ref{data_stats} that overlap of utterances with their class-label name is highest for ATIS and lowest for NLUED dataset. Additionally, the size of label space, both for seen and novel classes is smaller for ATIS than NLUED dataset. However, contrary to the expectation, ATIS 

\subsection{Label-wise Performance}
\label{label_wise}

For further analysis of the performance of the model, we study the label-wise results for both FSID and GFSID setting. We present label-wise results for SNIPS dataset in Table \ref{snips_label_wise}. We do not show results for all datasets for the sake of brevity. However, we can common observations across the datasets as mentioned below:
\begin{itemize}
    \item In general, the results of novel classes (\textit{add\_to\_playlist, rate\_book} for SNIPS) in GFSID settings drop compared to FSID settings. It shows that that the performance of model drops on novel classes in joint label space, which is expected. However, in some cases the gap is quite huge (\textit{play\_music} has a difference of 48\% in 1-shot FSID vs 1-shot GFSID). 
    Additionally, this drop is higher in case of 1-shot evaluation against 5-shot evaluation. This could be explained by the inherent difficulty of 1-shot setting as compared to 5-shot setting where the model has to learn from single example.
    
    \item Further analysis suggests that there is no correlation between the results on a specific label and its overlap with respective utterances. For example, a base intent \textit{get\_weather} has minimal overlap with utterances of this intent, has a similar performance as another base intent \textit{book weather} with a much higher overlap. Similarly, a novel intent \textit{rate\_book} has lowest (among novel classes) exact match and unordered match percentage between class-label name and respective utterances, but has better performance than \textit{add\_to\_playlist,  play\_music} intents which have higher unordered match. The pattern of these observations hold true with datasets with larger number of labels as well (NLUED, BANKING77, CLINC150). 
    % The detailed label-wise tables are not shown for sake of brevity. 
    These results indicate that model does not learn a trivial rule of matching the overlap between utterance and class-label name, but is using semantic associations to identify if an utterance entails an intent. Qualitative analysis presented in next sub-section supports this finding,  where even with an utterance containing exact class-label name results in an incorrect prediction in some cases.
\end{itemize}

\begin{table*}[h]
\centering
\small

\begin{tabular}{l|ll|ll|cc}
\multirow{2}{*}{\textbf{Intents}} & \multicolumn{2}{c|}{\textbf{1-shot}} & \multicolumn{2}{c|}{\textbf{5-shot}} & \multirow{2}{*}{\textbf{\begin{tabular}[c]{@{}c@{}}Exact \\ Match \%\end{tabular}}} & \multirow{2}{*}{\textbf{\begin{tabular}[c]{@{}c@{}}Unordered\\ Match \%\end{tabular}}} \\ \cline{2-5}
                                  & FSID              & GFSID            & FSID              & GFSID            &                                                                                     &                                                                                        \\ \hline
\textit{add to playlist}          & 87.97             & 57.72            & 86.70             & 77.98            & 0                                                                                   & 49.08                                                                                  \\
\textit{book restaurant}          & \_                & 93.47            & \_                & 96.37            & 0.05                                                                                & 26.21                                                                                  \\
\textit{get weather}              & \_                & 98.28            & \_                & 94.59            & 0                                                                                   & 0.2                                                                                    \\
\textit{play music}               & 78.67             & 30.39            & 91.51             & 88.36            & 8.86                                                                                & 25.06                                                                                  \\
\textit{rate book}                & 90.56             & 79.89            & 92.29             & 85.71            & 0                                                                                   & 11.08                                                                                  \\
\textit{search creative work}     & \_                & 74.44            & \_                & 74.02            & 0                                                                                   & 0                                                                                      \\
\textit{search screening event}   & \_                & 86.05            & \_                & 85.89            & 0                                                                                   & 0                                                                                     
\end{tabular}
\caption{Label-wise macro F1-score for SNIPS dataset. "-" in FSID column denotes that the respective classes are considered as base class.}
\label{snips_label_wise}
\end{table*}

\subsection{Qualitative Examples}
\label{qual}

\begin{table*}[h]
\centering
\small

\begin{tabular}{llll}
\textbf{Sl. No.} & \textbf{Example Utterance}                                           & \textbf{Gold Label}  & \textbf{\begin{tabular}[c]{@{}l@{}}Predicted Intent \\ (NLI-FSL)\end{tabular}} \\ \hline
1                & \textit{book a restaurant with parking facility for 3}               & book restaurant      & book restaurant                                                                \\
2                & \textit{play some alternative music on vimeo}                        & play music           & play music                                                                     \\
3                & \textit{add artist hex hector to my old school death metal playlist} & add to playlist      & add to playlist                                                                \\
                 & \textit{}                                                            &                      &                                                                                \\
4                & \textit{please find the album the party scene}                       & search creative work & search creative work                                                           \\
5                & \textit{i need a reservation for ten at a tavern in west virginia}   & book restaurant      & book restaurant                                                                \\ \hline
                 & \textit{}                                                            &                      &                                                                                \\
6                & \textit{list out what is on my shopping list}     & shopping list      & shopping list update                                                                      \\

7                & \textit{skip to the next song please}     & next song      & update playlist                                                                      \\
                 & \textit{}                                                            &                      &                                                                                \\

8                & \textit{show me the movie haunted spooks}                            & search creative work & search screening event                                                         \\
9                & \textit{go ahead and hold a conference room for friday at 11 am}                                                & schedule meeting           & schedule maintenance                                                           \\
% 9                & \textit{show olympia 81 saga}                                        & search creative work & get weather                                                                    \\
10                 & \textit{play my hype playlist on youtube}                            & play music           & add to playlist        \\ \hline   
                %  & \textit{}                                                            &                      &                                                                                \\
                %  & \textit{schedule}                         & book restaurant      & rate book                                                                      \\
                %  & \textit{play my hype playlist on youtube}                            & play music           & add to playlist        \\ \hline                                                       
\end{tabular}
\caption{Representative examples where the NLI-FSL model predicts correct and incorrect intents for a given utterance.}
\label{examples}
\end{table*}

In order to do an in-depth study of the predictions by NLI-FSL model, we do an error analysis by analyzing the predictions from the model. We sample a total of 100 datapoints (utterances) across the datasets, 50 each from correct and incorrect predictions. Table \ref{examples} provide an overview of representative examples of the two cases. The observations from error analysis can be described as:

\begin{itemize}
    \item \textbf{Cases where predictions from models are correct}: Examples 1-5 presents utterances and corresponding intent where the predicted intent from model matches the gold class-label. On a closer look, we further divide these utterances into two buckets: i) categories of intents that has overlap (exact or unordered) with the utterance (example 1-3), and, ii) bucket where the overlap between intent and utterance is absent (example 4-5). Out of a total of 50 sampled utterances with correct predictions, a majority of cases (86\%) belong to the latter bucket, thus showing that model is able to identify the correct intents by the contrasting the positive and negative pairs.
    
    \item \textbf{Cases where predictions from models are incorrect}: Incorrect predictions are represented by examples 6-10 in Table \ref{examples}. As mentioned above, here, we again study the errors into two intuitive buckets: the bucket where utterance and class-label overlap and the bucket where they don't have a token overlap. While it is not expected from the model to make mistakes on the simpler case when there is a overlap between utterance and class-label, it can be noted that the predicted intent in both examples hold a similar semantics with the gold class-label. We conjecture that model may be confused between the labels having higher semantic associations and thus predicts a wrong intent. The remaining examples with incorrect predictions corroborates previous finding where the predicted intent and gold label have a higher level association of user's goals (eg: the intent is to set up an appointment in both \textit{schedule meeting} and \textit{schedule maintenance}). To resolve some of these errors, we would want to study an intelligent sampling technique during the data transformation step that generates negative samples from closely matching intents. We hope that model would then be able to discriminate close intents with a better than currently observed performance.
\end{itemize}

% \section{Confusion Matrix for Generalized Few-Shot}

% \input{latex/introduction}
% \input{latex/problem}
% \input{latex/methodology}
% \input{latex/data_and_baselines}
% \input{latex/Exp_and_result}
% \input{latex/related}
% \input{latex/conclusion}

% \bibliography{anthology,custom}
% \bibliographystyle{acl_natbib}

% \appendix
